# Supplementary material for: Toward generative machine learning for boosting ensembles of climate simulations
Source: arXiv:2602.06287 source file (2026-02-06)
Supplement: Supplementary file 1 [file SI_Toward_generative_machine_learning_for_boosting_the_ensembles_size_of_climate_simulation.pdf]

# Supporting Information for "Toward generative machine learning for boosting ensembles of climate simulations"

Parsa Gooya<sup>1</sup>,Reinel Sospedra-Alfonso<sup>1</sup>, and Johannes Exenberger<sup>2,3</sup>

<sup>1</sup>Canadian Centre for Climate Modeling and Analysis, Environment and Climate Change Canada, Victoria, British Columbia,

Canada

<sup>2</sup>Vienna University of Technology

<sup>3</sup>Institute of Software Technology and Artificial Intelligence, Graz University of Technology

## Contents of this file

1. Text S1 to S2

2. Figures S1 to S9

3. Tables S1 to S2

**Introduction** The Supporting Information provides details of the derivation of the Evidence Lower Bound (ELBO) for training the conditional Variation Autoencoder (cVAE) model used for this study, as well as the architectural details of the models. Supporting figures S1 to S9 provide complementary analysis and/or deeper insight to the main analysis as referenced in the main text.

## S1. Evidence Lower Bound (ELBO)

The Evidence Lower Bound used as the objective function to train the cVAE models is derived to maximize a *lower bound* to the conditional log-likelihood over the dataset  $\{x_i\}_{i=1}^I$  for the modeled distribution. In other words, the goal is to optimize the parameters of the model that parametrize the distribution  $p(x|c)$  in a way that the log-likelihood over the dataset is maximized. We formulate this using the latent variable  $z \sim p(z|c)$ . For each data point  $x_i$  (in this case maps of climate variables) with it corresponding condition  $c_i$ :

$$\log[p(x_i|c_i)] = \log \left[ \int p(x_i, z|c_i) dz \right] = \log \left[ \int q(z|c_i) \frac{p(x_i, z|c_i)}{q(z|c_i)} dz \right] \quad (1)$$

where we multiplied and divided the likelihood by an arbitrary probability distribution  $q(z|c_i)$ . The multiplication might look arbitrary but intuitively it is built on the idea of importance sampling, as integrating over the entirety of the  $\mathcal{Z}$  space is inefficient given that likely only a sub-region of the space will contribute to the most likely reconstructions of sample  $x_i$ . Using Jensen's inequality we can drive the lower bound as:

$$\log[p(x_i|c_i)] \geq \int q(z|c_i) \log \left[ \frac{p(x_i, z|c_i)}{q(z|c_i)} \right] dz \quad (ELBO) \quad (2)$$

The ELBO can thus be written as:

$$\begin{aligned}
ELBO &= \int q(z|c_i) \log \left[ \frac{p(x_i, z|c_i)}{q(z|c_i)} \right] dz \\
&= \int q(z|c_i) \log \left[ \frac{p(x_i|z, c_i)p(z|c_i)}{q(z|c_i)} \right] dz \\
&= \int q(z|c_i) \log [p(x_i|z, c_i)] dz + \int q(z|c_i) \log \left[ \frac{p(z|c_i)}{q(z|c_i)} \right] dz \\
&= \mathbb{E}_{F \sim \Pi(F|\Xi)} [\log [p(x_i|z, c_i)]] - D_{KL} [q(z|c_i) || p(z|c_i)] \tag{3}
\end{aligned}$$

30 Note that we used the expectation  $\mathbb{E}_{z \sim q(z|c_i)} [f(z)]$  in place of the integral  $\int f(z)q(z|c_i)dz$   
 31 and the definition of Kullback–Leibler Divergence for the second term. The best choice for  
 32  $q(z|c_i)$  to inform the sampling of the  $\mathcal{Z}$  space is the posterior distribution  $p(z|x_i, c_i)$ . It can  
 33 be shown that this would actually close the inequality and make the ELBO equal to the  
 34 log-likelihood (see Equation 17.17 from Prince (2023)). However,  $p(z|x_i, c_i)$  is intractable  
 35 and would require, via the Bayes’ rule, the calculation of  $p(x_i|c_i)$  which is what we are  
 36 trying to model in the first place. Thus, we use the encoder to parametrize a Gaussian  
 37 distribution  $q_\phi(z|x_i, c_i)$  that approximates the true posterior with  $\phi$  being the parameters  
 38 of the encoder neural network.

39 By parameterizing the distribution  $p(x_i|z, c_i)$  with a decoder neural network of param-  
 40 eters  $\theta$ , the ELBO can be written as,

$$ELBO(\theta, \phi) = E_{q_\phi(z|x_i, c_i)} [\log p_\theta(x_i|z, c_i)] - KL(q_\phi(z|x_i, c_i) || p(z|c_i)) \tag{4}$$

41 Although the first term in the ELBO is intractable, it is an expectation over the known  
 42 distribution  $q_\phi(z|x_i, c_i)$  of a functional of the parameterized generative model, and can be  
 43 approximated using Monte Carlo sampling:

$$\mathbb{E}_{q_\phi(z|x_i, c_i)} [\log p_\theta(x_i|z, c_i)] = \frac{1}{L} \sum_{l=1}^L \log p_\theta(x_i|z_l, c_i) \quad , \quad z_l \sim q_\phi(z|x_i, c_i) \tag{5}$$

Therefore, by using the parameterization of the decoder distribution provided in Eq. 3 in terms of a Gaussian ( $\mathcal{N}(\mu_{NN_\theta}(z, c), \sigma^2 I)$ ), the log-likelihood of data sample  $x_i$  can be written in the closed form:

$$\log p_\theta(x_i|z, c_i) = \sum_{n=1}^N \left[ -\frac{\log \sigma^2}{2} - \frac{\log(2\pi)}{2} - \frac{\|\mu_{NN_\theta}(z, c_i) - x_i\|^2}{2\sigma^2} \right] \quad (6)$$

where  $N$  is the dimension of the output  $x_i$ . Given that the first two terms are independent of the model parameters  $\theta$ , the optimization of the log-likelihood is equivalent to minimizing the MSE of the output. The learning objective is thus maximizing the ELBO which is equivalent to minimizing the following loss function:

$$\text{Min}_{\theta, \phi} \quad J(\theta, \phi) = \text{MSE}(\mu_{NN_\theta}(z, c_i), x_i) + \beta \text{KL}(q_\phi(z|x_i, c_i) \| p(z|c_i)) \quad (7)$$

Finally, training with this loss function includes sampling the posterior distribution  $q_\phi(z|x_i, c_i)$ . This is a random process which inhibits back-propagation of gradients. To address this, the reparameterization trick was introduced (Kingma & Welling, 2022) with the latent variable  $z_l$  is expressed as:

$$z_l = g_\phi(x, c, \epsilon_l) = \mu_{NN_\phi}(x, c) + \sigma_{NN_\phi}(x, c)\epsilon_l, \quad \epsilon_l \sim \mathcal{N}(0, I), \quad (8)$$

Here  $g_\phi$  is a deterministic function of  $q_\phi(z|x, c)$  Gaussian parameters reparameterizing the randomness in sampling the posterior by the use of  $\epsilon$ . As a result, the cVAE can be efficiently optimized using stochastic gradient decent. In the original derivation,  $\beta = 1$ , but one can weigh the  $KL$  term with positive values for  $\beta$  to come up with the optimal trade-off between reconstruction quality and latent space regularization. This is essential for a successful generative model with meaningful and structured latent space (Higgins et al., 2017) and is a hyperparameter of the model.

## S2. Model architecture and training details

The model architecture used for this study is based on MLPs, which are series of dense layers followed by ReLU activation. The input TAS maps are of  $64 \times 128 = 8192$  in size. The encoder consecutively decreases the dimension of the input to the  $z \in \mathbb{R}^{500}$  latent space (Table 1) and outputs the  $\mu_{NN_\phi}$  and  $\log \sigma_{NN_\phi}^2$  of the  $q_\phi(z|x_i, c_i)$  distribution (Equation 4). The decoder reverses encoder steps using samples generated from the latent space (Table 2). For condition embedding, we use a separate MLP denoted  $F_{NN}(x_i)$  with the same architecture as the encoder but with an embedding vector  $c_i \in \mathbb{R}^2$  passed to both the decoder and encoder. Finally, the encoder receives both the input  $x_i$  and condition  $c_i$ , while the decoder receives samples from the latent space together with the condition  $c_i$  concatenated to the first layer of the decoder. All three MLPs are trained end-to-end.

All models are trained using the Adam optimizer, a learning rate of 0.0001, and batch size of 100. Since that the ELBO loss is the combination of a log-likelihood (MSE) term and  $KL$  divergence term, both of which are calculated for distributions that are parametrized as multinormal with diagonal covariances, both losses should be summed over all of the dimensions of the corresponding distributions, i.e., the latent dimensions for the  $KL$  term and decoder dimensions (same as image dimensions) for the log-likelihood (MSE) term. We normalized both terms in the loss function based on the dimensionality of the corresponding distribution and chose the proper  $\beta$  to adjust the contribution of the two terms. We chose 0.1 for  $\beta$  given than the input dimensionality is of  $o(10)$  compared to that of the latent vector. All models were trained for 100 epochs with beta annealing (Sankarapandian & Kulis, 2021) by linearly increasing the  $\beta$  weight of the  $KL$  term in the loss function from zero to 0.1 over the first 10 epochs. For this study, we did not perform any hyperparameter tuning besides the embedding vector size. The performance was measured based on the reconstruction quality by Monte Carlo sampling over 2020-2025

time period that was withheld as validation. However, we did not find much sensitivity to the choice of  $\beta$  as long as it was not too large that the  $KL$  loss dominates the training and the model experiences a *posterior collapse*, i.e., the posterior becoming indistinguishable from the prior distribution (standard Gaussian) and the model essentially ignoring the latent space.

## References

- Higgins, I., Matthey, L., Pal, A., Burgess, C., Glorot, X., Botvinick, M., ... Lerchner, A. (2017). beta-VAE: Learning basic visual concepts with a constrained variational framework. In *International conference on learning representations*. Retrieved from <https://openreview.net/forum?id=Sy2fzU9g1>
- Kingma, D. P., & Welling, M. (2022). *Auto-encoding variational bayes*. Retrieved from <https://arxiv.org/abs/1312.6114>
- Sankarapandian, S., & Kulis, B. (2021).  *$\beta$ -annealed variational autoencoder for glitches*. Retrieved from <https://arxiv.org/abs/2107.10667>

| Layer | Operation                                                                                 | Size-in                                                  | Size-out                                   |
|-------|-------------------------------------------------------------------------------------------|----------------------------------------------------------|--------------------------------------------|
| 1     | Flatten                                                                                   | $batch \times 64 \times 128$                             | $batch \times 8192$                        |
| 2     | Dense<br>ReLU                                                                             | $batch \times (8192 + condition)$<br>$batch \times 3000$ | $batch \times 3000$<br>$batch \times 3000$ |
| 4–6   | Dense + ReLU                                                                              | $batch \times 3000$                                      | $batch \times 3000$                        |
| 7     | Dense ( $\mu$ )<br>Dense ( $\log \sigma^2$ )                                              | $batch \times 3000$<br>$batch \times 3000$               | $batch \times 500$<br>$batch \times 500$   |
| 8     | Reparameterization: $z = \mu + \sigma \cdot \epsilon$ , $\epsilon \sim \mathcal{N}(0, I)$ | —                                                        | $batch \times 500$                         |

**Table S1.** Encoder MLP. The input is flattened first, and the cVAE, the embedding of the condition (size 2) is concatenated before the first dense layer. Layers 4–6 represent repeated Dense+ReLU blocks. Layer 7 outputs the distribution parameters, and layer 8 applies the reparameterization trick. Note that there is no activation in layer 7.

| Layer | Operation          | Size-in                                                 | Size-out                                            |
|-------|--------------------|---------------------------------------------------------|-----------------------------------------------------|
| 1     | Dense<br>ReLU      | $batch \times (500 + condition)$<br>$batch \times 3000$ | $batch \times 3000$<br>$batch \times 3000$          |
| 2–6   | Dense<br>ReLU      | $batch \times 3000$<br>$batch \times 3000$              | $batch \times 3000$<br>$batch \times 3000$          |
| 7     | Dense<br>Unflatten | $batch \times 3000$<br>$batch \times 8192$              | $batch \times 8192$<br>$batch \times 64 \times 128$ |

**Table S2.** Decoder MLP. The condition embedding is concatenated to the first layer of the decoder. Note that there is no activation in layer 7.

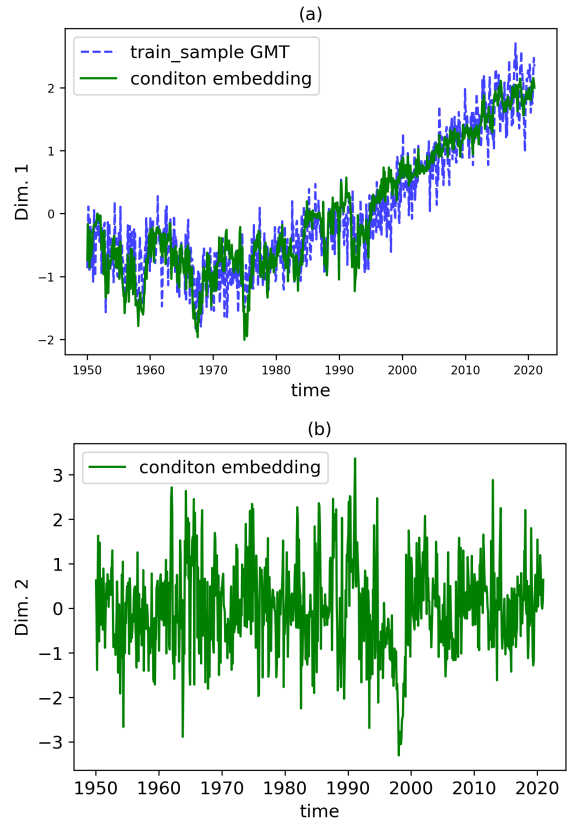

**Figure S1.** a) Time series of the first PC (principle component) of the condition embedding vector  $c \in \mathbb{R}^2$  from training snapshots. Also plotted is the time-series of the globally averaged TAS anomaly (GMT) from train sample. Both time series are standardized to have similar scales. (b) Time series of the second PC of the condition embedding vector  $c \in \mathbb{R}^2$ . There is close agreement between the two time-series on panel (a) with smaller variability on the condition embedding vector indicating filtering out of the noise specific to the training realization.

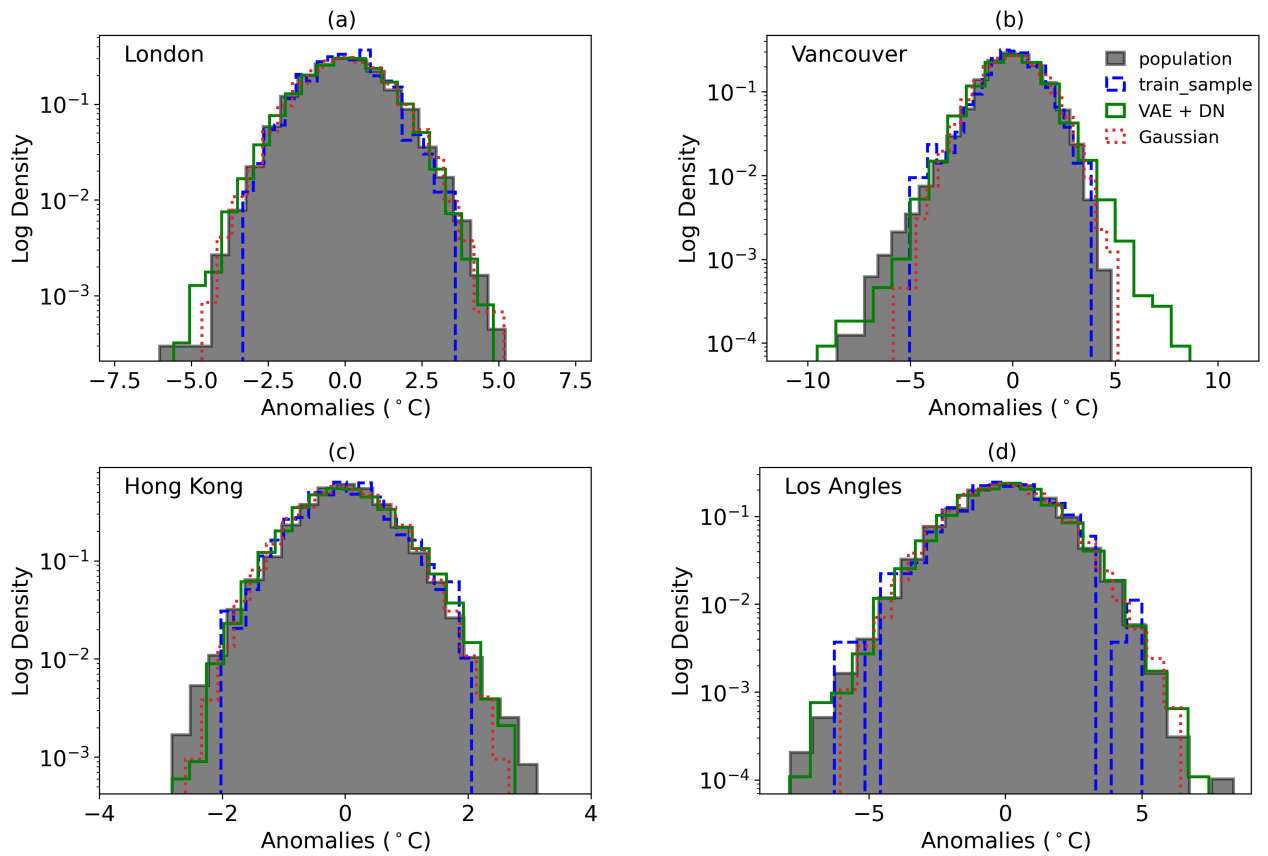

**Figure S2.** PDF plots on log scale for the four cities with the addition of the Gaussian fit to the population. Note that this Gaussian is not available to us since we do not have access to the population statistics and this is only to show the difference from non-Gaussian behavior.

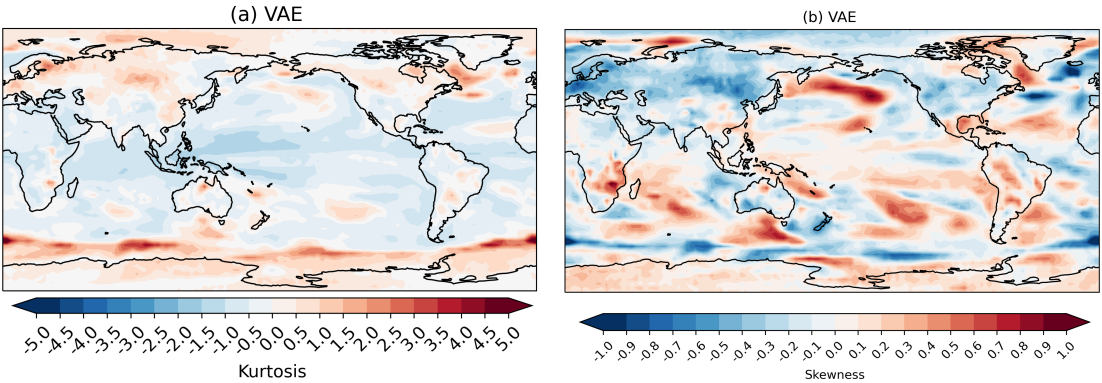

**Figure S3.** a) Kurtosis and b) Skewness of the TAS anomalies distributions from the VAE model without decoder noise sampling.

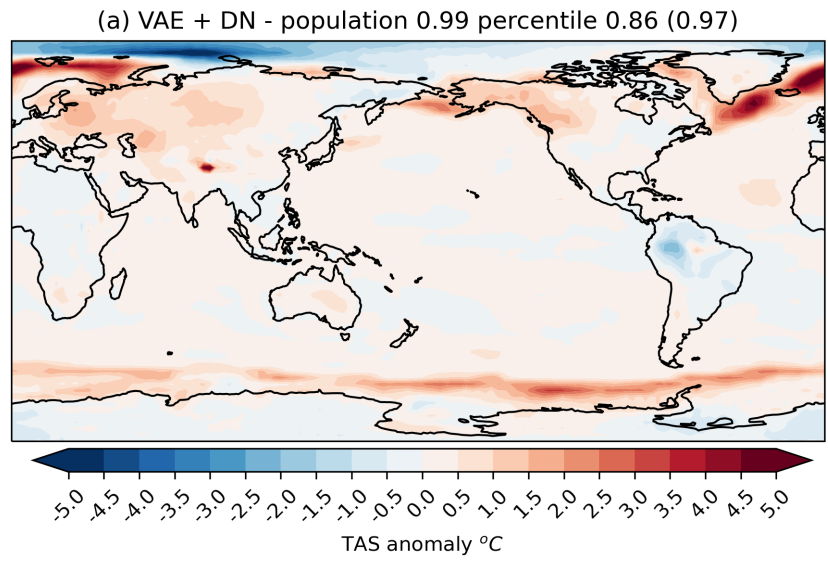

**Figure S4.** Difference between VAE+DN and population in %99 percentile TAS anomalies. The numbers in the label are RMSE (pattern correlation) between VAE+DN and population.

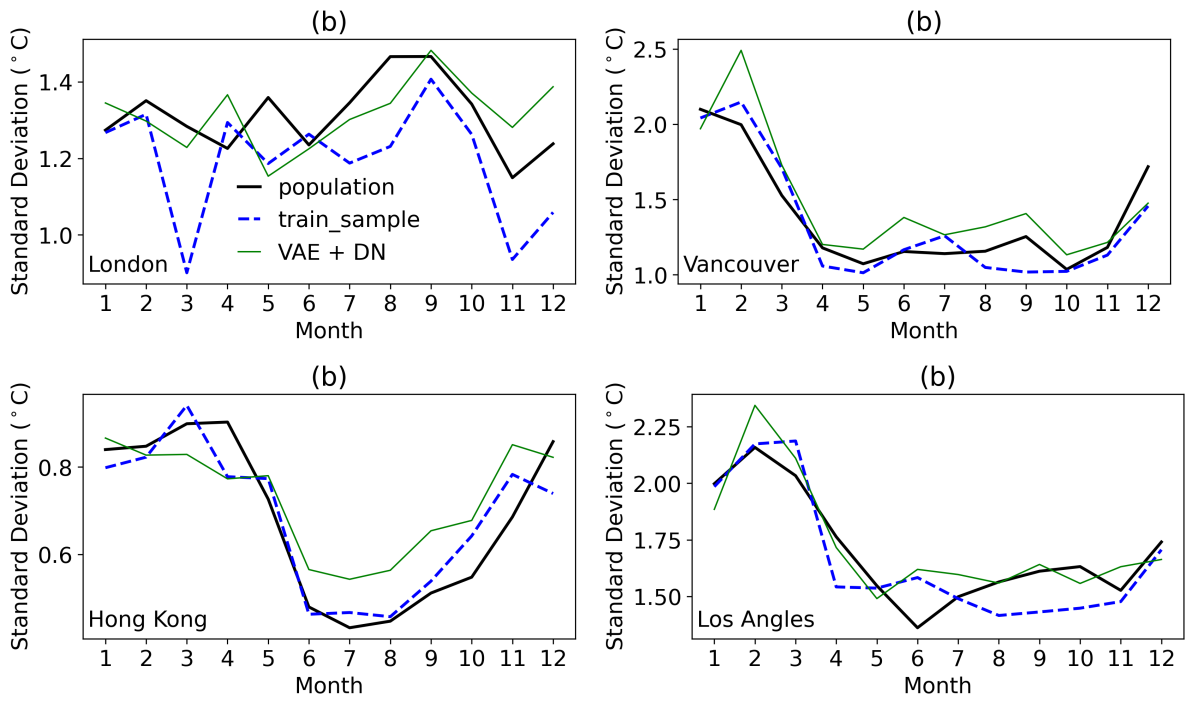

**Figure S5.** Time series of seasonal standard deviation of TAS anomalies over London, Vancouver, Hong Kong, and Los Angeles.

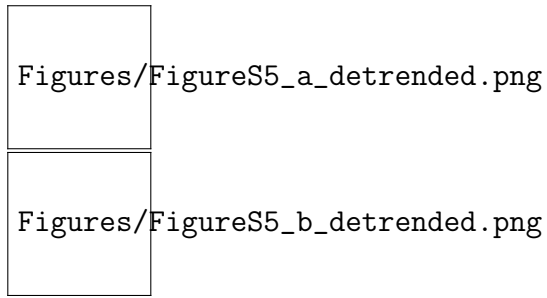

**Figure S6.** Composites of the linearly detrended monthly TAS anomalies for El-Niño events classified using the 75<sup>th</sup>, 85<sup>th</sup> percentiles based on the Niño3.4 index from the training sample. Numbers in the title are pattern correlation with the corresponding population.

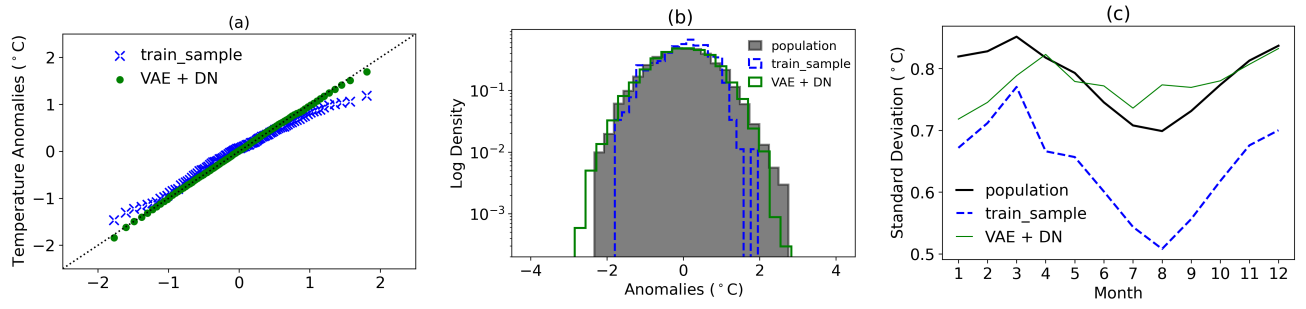

**Figure S7.** a) QQ plots (b) PDF and (c) seasonal cycle of variability in Niño3.4 index based on detrended TAS fields for different data products

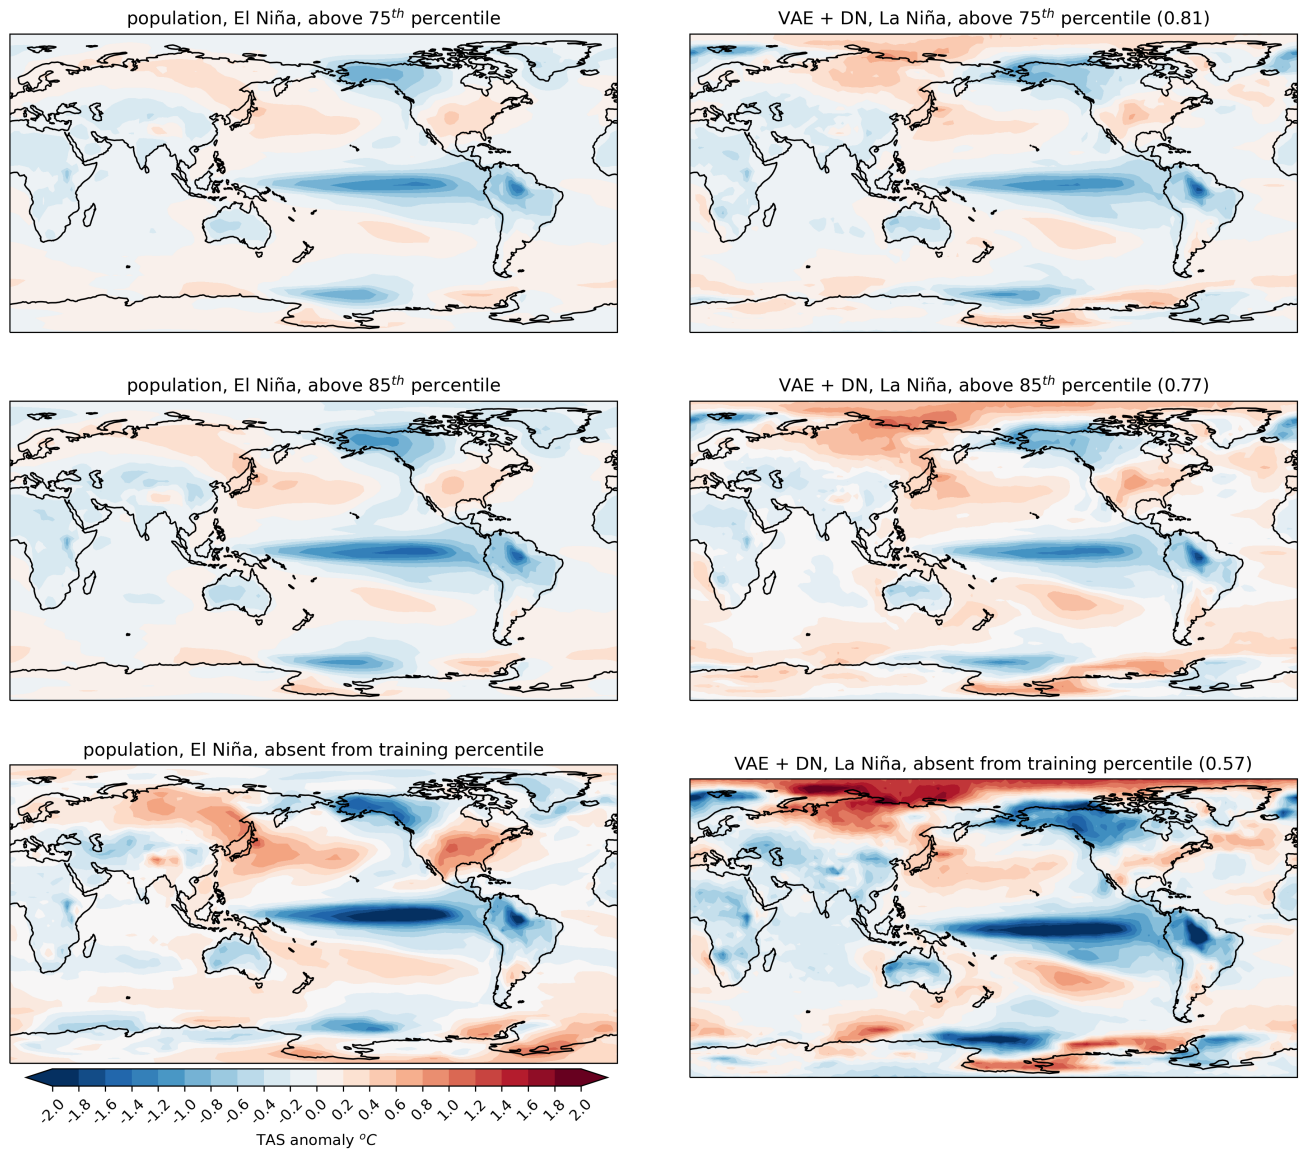

**Figure S8.** Composites of the linearly detrended monthly TAS anomalies for La-Niña events classified using the 75<sup>th</sup>, 85<sup>th</sup> and absent from training percentiles based on the Niño3.4 index (rows). First column is the population dataset and the second column is the boosted ensemble from VAE+DN model.

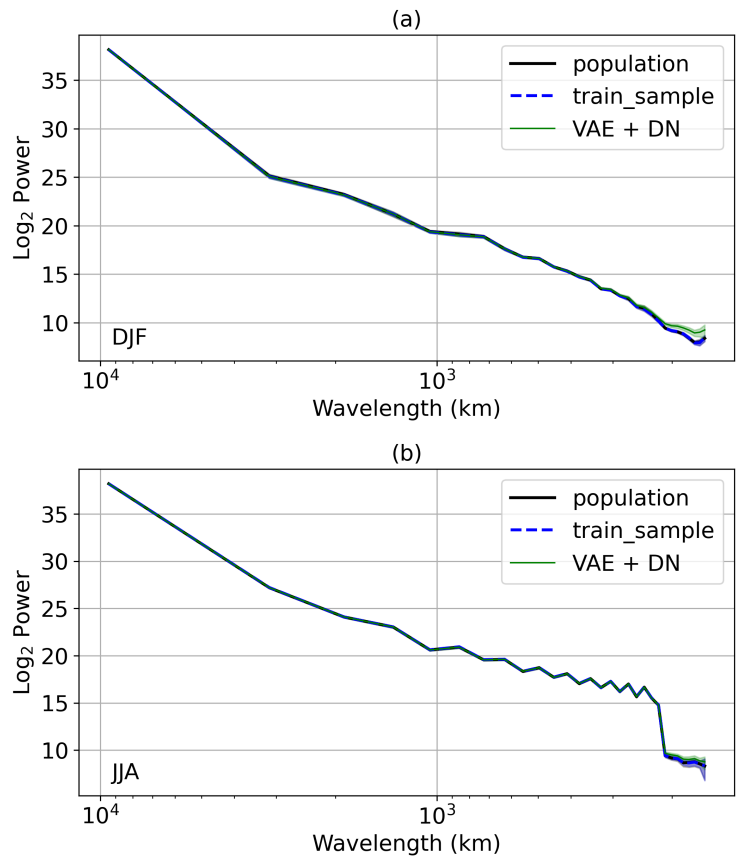

**Figure S9.** Radially averaged power spectra for DJF and JJA averaged over 1980-2020 across ensemble members for population, train, and VAE + DN datasets.
